# Supplementary material for: VecCity: A Taxonomy-guided Library for Map Entity Representation Learning
Source: arXiv:2411.00874 source file (2025-05-07)
Supplement: Supplementary file 1 [file 6-appendix.tex]

\section{Appendix}

\paratitle{Model Architecture.} To eliminate the influence of model architecture on the final results, we use the same encoder within each type of model and include only the necessary encoding components. Specifically:
\begin{itemize}[leftmargin=*]
    \item {\em Token Encoder:} A simple, learnable embedding layer is used to convert entity IDs into token representations. Specifically, the token encoder for POI incorporates spatial features by transforming coordinates (latitude and longitude) into a vector using an MLP, while the land parcel encoder integrates POI feature information in a similar way.
    \item {\em Graph Encoder:} Graph Convolution Network (GCN) is employed to encode auxiliary data associated with the graph-based task. For land parcels, the relation network considers POI similarity, spatial distance, and mobility as edge weights, following the approach used in HREP~\citeNew{HREP}.
    \item {\em Sequence Encoder:} A Transformer layer is utilized to encode data corresponding to the sequence-based pretraining task.
\end{itemize}

The model parameters are configured as follows:
% \begin{table*}[t]
% \centering
%     \caption{Model settings.}
%     \renewcommand{\arraystretch}{1} % Adjust row height for better readability
%     \begin{tabular}{l|c||l|c}
%     \hline
%     \textbf{Parameter}               & \textbf{Value} & \textbf{Parameter}            & \textbf{Value} \\ \hline
%     Learning Rate                    & 1e-3           & Embedding Dimension           & 128            \\ \hline
%     Hidden Dimension                 & 256            & Max Check-in Trajectory Length       & 32             \\ \hline
%     Max Coordinates Trajectory Length      & 128            & Train-Valid-Test Ratio              & 6:2:2            \\ \hline
%     Number of Training Steps         & 50,000         &                               &                \\ \hline
%     \end{tabular}
%     \label{tab:model_parameters_dual_column}
% \end{table*}
\begin{table}
\centering
\caption{Model settings.}
 % Row height for readability
\begin{tabular}{l|c}
\hline
\textbf{Parameter} & \textbf{Value} \\ \hline
Learning Rate & 1e-3 \\
Embedding Dimension & 128 \\
Hidden Dimension & 256 \\
Max Check-in Trajectory Length & 32 \\
Max Coordinates Trajectory Length & 128 \\
Train-Valid-Test Ratio & 6:2:2 \\
Number of Training Steps & 50,000 \\
\hline
\end{tabular}
\label{tab:model_parameters_single_column}
\end{table}

As discussed in Section~\ref{sec:taxonomy_pretraining}, the model organizes the different types of encoders in the commonly used order: Token → Graph → Sequence.

\paratitle{Static Information of the City Dataset.}
For clarity, we provide a detailed overview of the datasets in \tab\ref{tab:newdataset}. In addition to the original information, we incorporate visit frequency (Freq). Visit frequency represents the number of records associated with each map entity.

% Table generated by Excel2LaTeX from sheet 'data'
\begin{table*}
  \centering
  \caption{Pre-prepared datasets for \fullname.}
  \setlength{\tabcolsep}{0.8mm}
  \resizebox{0.7\textwidth}{!}{
    \begin{tabular}{l|rrr|rrr|rrr|r}
    \toprule
    \multirow{2}{*}{City} & \multicolumn{1}{c}{\multirow{2}{*}{\#POI}} & \multicolumn{1}{c}{\multirow{2}{*}{\#Segment}} & \multicolumn{1}{c|}{\multirow{2}{*}{\#Parcel}} & \multicolumn{3}{c|}{Check-in Traj} & \multicolumn{3}{c|}{Coor. Traj} & \multicolumn{1}{c}{\multirow{2}{*}{\#OD}} \\
\cline{5-10}          &       &       &       & \multicolumn{1}{c}{\#Traj} & \multicolumn{1}{c}{\#User} & \multicolumn{1}{c|}{Freq} & \multicolumn{1}{c}{\#Traj} & \multicolumn{1}{c}{\#User} & \multicolumn{1}{c|}{Freq} &  \\
    \midrule
    NY    & 79,627 & 90,781 & 262   & 823,853 & 2,758 & 30    & \multicolumn{1}{c}{--}     & \multicolumn{1}{c}{--}     & \multicolumn{1}{c|}{--}     & 28,189 \\
    CHI   & 28,141 & 47,669 & 77    & 279,183 & 921   & 57    & \multicolumn{1}{c}{--}     & \multicolumn{1}{c}{--}     & \multicolumn{1}{c|}{--}     & 4,631 \\
    TYO   & 61,858 & 407,905 & 64    & 823,853 & 2,227 & 29    & \multicolumn{1}{c}{--}     & \multicolumn{1}{c}{--}     & \multicolumn{1}{c|}{--}     & \multicolumn{1}{c}{--} \\
    SIN   & 75,329 & 35,084 & 332   & 827,828 & 3,489 & 49    & 226,782 & None  & 35    & \multicolumn{1}{c}{--} \\
    PRT   & 4,521 & 11,095 & 382   & 19,402 & 126   & 9     & 695,085 & 435   & 2,430 & 324 \\
    SF    & 15,674 & 27,274 & 194   & 171,873 & 361   & 23    & 500,516 & 405   & 771   & 24,716 \\
    BJ    & 81,181 & 40,306 & 11,208 & \multicolumn{1}{c}{--}     & \multicolumn{1}{c}{--}     & \multicolumn{1}{c|}{--}     & 1,018,312 & 1,677 & 856   & 687,890 \\
    CD    & 17,301 & 6,195 & 1,306 & \multicolumn{1}{c}{--}     & \multicolumn{1}{c}{--}     & \multicolumn{1}{c|}{--}     & 559,729 & 48,295 & 1,551 & 64,482 \\
    XA    & 19,108 & 5,269 & 1,056 & \multicolumn{1}{c}{--}     & \multicolumn{1}{c}{--}     & \multicolumn{1}{c|}{--}     & 384,618 & 26,787 & 1,359 & 54,365 \\
    \bottomrule
    \end{tabular}%
    }
  \label{tab:newdataset}%
\end{table*}%

\paratitle{Performance Analysis.} 
The complete experimental results are presented in \tab\ref{tab:poi_comb} for POI, \tab\ref{tab:road_segment_comb} for road segment, and \tab\ref{tab:land_parcel_comb} for land parcel. To facilitate comparison, we also highlight the Top 3 task combinations based on the average ranking across tasks and datasets in \fig\ref{fig:comb}, where each subfigure corresponds to a specific downstream task or dataset. The horizontal axis shows the ranking (lower is better), and the vertical axis lists the top three combinations, with lighter colors indicating lower ranks. In \fig~\ref{fig:comb}(a) for POI entities, the first three subfigures show each model’s average ranking in a specific downstream task (POIC, NPP, or TUL) across multiple datasets. We refer to these as {\em task-oriented rankings}. In contrast, the last five subfigures show each model’s average ranking across all tasks within a specific dataset (NY, TYO, CHI, SIN, or SF), which we refer to as {\em dataset-oriented rankings}. The same ranking logic applies to \fig~\ref{fig:comb}(b) for road segments and \fig~\ref{fig:comb}(c) for land parcels. Based on the results, we have several key findings:

1) {\em Optimal Combinations for POI:}
TokRI + MTR consistently ranks highest, likely due to its ability to model POI categories and sequence dependencies—two key attributes for POIs. However, in SF, where data sparsity is more pronounced, TokRI + TrajP emerges as a more suitable alternative, as TrajP focuses on local sequential patterns, making it more reliable in sparse data scenarios.

2) {\em Optimal Combinations for Road Segment:}
AGCL outperforms others in all scenarios, as it effectively captures important spatial dependencies in geographic relation networks, which is critical for modeling road segments. From a dataset-oriented perspective, AGCL + MTR achieves the best results in CD and PRT, where visit frequencies are higher (CD: 1551, PRT: 2430), allowing MTR to learn sequential dependencies from dense trajectory data. In contrast, AGCL + TrajP works better in BJ and SF, where visit frequencies are lower (BJ: 856, SF: 771). This suggests that MTR benefits more from dense data, while TrajP is better suited for sparse data.

3) {\em Optimal Combinations for Land Parcel:}
AToCL achieves the best performance in 5/8 cases, likely because its augmentation technique enhances the model’s ability to capture key semantic features while filtering out noise. This is especially important for land parcels, where POI category distributions define functional attributes. GAu and NFI are also well-suited for land parcels, as they better model similarity-driven connectivity in social relation networks.

\paratitle{Complete Performance Comparison of Pretraining Task Combinations.} The full results for POI are presented in \tab~\ref{tab:poi_comb}, while \tab~\ref{tab:road_segment_comb} and \tab~\ref{tab:land_parcel_comb} provide the corresponding results for road segments and land parcels, respectively.
\begin{table}
  \centering
  \caption{Performance comparison of pretraining task combinations for POI across various datasets.}
      \resizebox{\linewidth}{!}{
      \setlength{\tabcolsep}{0.5mm}
       \setlength{\extrarowheight}{-1pt}
    \begin{tabular}{c|cc|ccc|ccc}
        \toprule
        \multicolumn{3}{c|}{Token-based} & \multicolumn{3}{c|}{TokRI} & \multicolumn{3}{c}{TRCL} \\
        \midrule
        \multicolumn{3}{c|}{Sequence-based} & TrajP & MTR   & ATrCL & TrajP & MTR   & ATrCL \\
        \midrule
        \multirow{6}[2]{*}{\rotatebox{90}{New York}} & \multicolumn{1}{c}{\multirow{2}[1]{*}{POIC}} & ACC@1↑ & \textbf{0.072} & \underline{0.072} & 0.062 & 0.055 & 0.059 & 0.057 \\
              & \multicolumn{1}{c}{} & F1↑   & \underline{0.005} & 0.003 & 0.004 & \textbf{0.006} & 0.004 & 0.004 \\
              & \multicolumn{1}{c}{\multirow{2}[0]{*}{NPP}} & ACC@1↑ & \underline{0.172} & \textbf{0.183} & 0.023 & 0.130 & 0.069 & 0.024 \\
              & \multicolumn{1}{c}{} & ACC@5↑ & \underline{0.363} & \textbf{0.392} & 0.050 & 0.275 & 0.164 & 0.060 \\
              & \multicolumn{1}{c}{\multirow{2}[1]{*}{TUL}} & ACC@1↑ & \underline{0.695} & \textbf{0.700} & 0.087 & 0.531 & 0.409 & 0.242 \\
              & \multicolumn{1}{c}{} & F1↑   & \underline{0.419} & \textbf{0.434} & 0.008 & 0.259 & 0.144 & 0.070 \\
        \midrule
        \multirow{6}[2]{*}{\rotatebox{90}{Tokyo}} & \multicolumn{1}{c}{\multirow{2}[1]{*}{POIC}} & ACC@1↑ & \underline{0.326} & \textbf{0.334} & 0.326 & 0.315 & 0.312 & 0.318 \\
              & \multicolumn{1}{c}{} & F1↑   & \underline{0.011} & \textbf{0.012} & 0.009 & 0.008 & 0.009 & 0.009 \\
              & \multicolumn{1}{c}{\multirow{2}[0]{*}{NPP}} & ACC@1↑ & \underline{0.187} & \textbf{0.197} & 0.059 & 0.045 & 0.060 & 0.037 \\
              & \multicolumn{1}{c}{} & ACC@5↑ & \underline{0.394} & \textbf{0.407} & 0.129 & 0.126 & 0.145 & 0.123 \\
              & \multicolumn{1}{c}{\multirow{2}[1]{*}{TUL}} & ACC@1↑ & \underline{0.501} & \textbf{0.527} & 0.040 & 0.050 & 0.155 & 0.032 \\
              & \multicolumn{1}{c}{} & F1↑  & \underline{0.281} & \textbf{0.307} & 0.006 & 0.010 & 0.049 & 0.004 \\
        \midrule
        \multirow{6}[2]{*}{\rotatebox{90}{Chicago}} & \multicolumn{1}{c}{\multirow{2}[1]{*}{POIC}} & ACC@1↑ & 0.233 & 0.242 & 0.218 & \textbf{0.280} & 0.251 & \underline{0.251} \\
              & \multicolumn{1}{c}{} & F1↑   & 0.068 & 0.076 & 0.068 & \textbf{0.094} & \underline{0.080} & 0.071 \\
              & \multicolumn{1}{c}{\multirow{2}[0]{*}{NPP}} & ACC@1↑ & \underline{0.181} & \textbf{0.209} & 0.031 & 0.063 & 0.122 & 0.045 \\
              & \multicolumn{1}{c}{} & ACC@5↑ & \underline{0.375} & \textbf{0.412} & 0.086 & 0.178 & 0.290 & 0.094 \\
              & \multicolumn{1}{c}{\multirow{2}[1]{*}{TUL}} & ACC@1↑ & \underline{0.734} & \textbf{0.771} & 0.170 & 0.262 & 0.588 & 0.262 \\
              & \multicolumn{1}{c}{} & F1↑   & \underline{0.543} & \textbf{0.611} & 0.013 & 0.055 & 0.346 & 0.049 \\
        \midrule
        \multirow{6}[2]{*}{\rotatebox{90}{Singapore}} & \multicolumn{1}{c}{\multirow{2}[1]{*}{POIC}} & ACC@1↑ & 0.126 & \textbf{0.140} & 0.126 & \underline{0.132} & 0.131 & 0.129 \\
              & \multicolumn{1}{c}{} & F1↑   & 0.003 & \textbf{0.004} & 0.003 & 0.004 & \underline{0.004} & 0.003 \\
              & \multicolumn{1}{c}{\multirow{2}[0]{*}{NPP}} & ACC@1↑ & \underline{0.113} & \textbf{0.114} & 0.011 & 0.035 & 0.046 & 0.020 \\
              & \multicolumn{1}{c}{} & ACC@5↑ & \textbf{0.254} & \underline{0.235} & 0.036 & 0.092 & 0.111 & 0.061 \\
              & \multicolumn{1}{c}{\multirow{2}[1]{*}{TUL}} & ACC@1↑ & \underline{0.454} & \textbf{0.455} & 0.016 & 0.217 & 0.264 & 0.107 \\
              & \multicolumn{1}{c}{} & F1↑   & \underline{0.215} & \textbf{0.215} & 0.000 & 0.075 & 0.099 & 0.011 \\
        \midrule
        \multirow{6}[2]{*}{\rotatebox{90}{San Francisco}} & \multicolumn{1}{c}{\multirow{2}[1]{*}{POIC}} & ACC@1↑ & \textbf{0.050} & 0.041 & 0.036 & \underline{0.045} & 0.041 & 0.041 \\
              & \multicolumn{1}{c}{} & F1↑   & \textbf{0.012} & 0.011 & 0.007 & \underline{0.012} & 0.007 & 0.010 \\
              & \multicolumn{1}{c}{\multirow{2}[0]{*}{NPP}} & ACC@1↑ & 0.147 & \textbf{0.161} & \underline{0.153} & 0.119 & 0.144 & 0.042 \\
              & \multicolumn{1}{c}{} & ACC@5↑ & \textbf{0.410} & \underline{0.370} & 0.314 & 0.291 & 0.339 & 0.116 \\
              & \multicolumn{1}{c}{\multirow{2}[1]{*}{TUL}} & ACC@1↑ & \textbf{0.777} & \underline{0.760} & 0.641 & 0.571 & 0.624 & 0.212 \\
              & \multicolumn{1}{c}{} & F1↑   & \underline{0.466} & \textbf{0.525} & 0.397 & 0.314 & 0.332 & 0.013 \\
        \midrule
        \multirow{2}{*}{Overall} & \multicolumn{2}{c|}{Per Ave Rank} & \underline{2.217} & \textbf{1.600} & 5.050 & 3.700 & 3.433 & 5.000 \\
              & \multicolumn{2}{c|}{Per Rank} & 2     & 1     & 6     & 4     & 3     & 5 \\
        \bottomrule
    \end{tabular}%
    }
  \label{tab:poi_comb}
\end{table}
\begin{table}
  \centering
  \caption{Performance comparison of pretraining task combinations for land parcel across various datasets.}
      \resizebox{\linewidth}{!}{
      \setlength{\tabcolsep}{0.3mm}
    \begin{tabular}{c|cc|ccc|ccc|ccc}
    \toprule
    \multicolumn{3}{c|}{Token-based} & \multicolumn{3}{c|}{TokRI} & \multicolumn{3}{c|}{TRCL} & \multicolumn{3}{c}{AToCL} \\
    \midrule
    \multicolumn{3}{c|}{Graph-based} & NFI   & GAu   & NCL   & NFI   & GAu   & NCL   & NFI   & GAu   & NCL \\
    \midrule
    \multirow{6}[2]{*}{\rotatebox{90}{Beijing}} & \multicolumn{1}{c|}{\multirow{2}[1]{*}{LPC}} & ACC@1↑ & \underline{0.528} & 0.430 & 0.376 & \textbf{0.538} & 0.480 & 0.370 & 0.464 & 0.360 & 0.366 \\
          & \multicolumn{1}{c|}{} & F1↑   & \underline{0.382} & 0.350 & 0.143 & \textbf{0.386} & 0.340 & 0.140 & 0.290 & 0.270 & 0.260 \\
          & \multicolumn{1}{c|}{\multirow{2}[0]{*}{FI}} & MAE↓  & \textbf{12.33} & 18.58 & 24.43 & 16.70 & 19.32 & 28.96 & \underline{13.71} & 16.51 & 25.18 \\
          & \multicolumn{1}{c|}{} & RMSE↓ & \textbf{40.17} & 63.73 & \underline{49.95} & 78.81 & 66.27 & 53.82 & 67.49 & 66.88 & 50.45 \\
          & \multicolumn{1}{c|}{\multirow{2}[1]{*}{MI}} & MAE↓  & \underline{0.272} & 0.340 & 0.292 & 0.394 & 0.290 & \textbf{0.257} & 0.279 & 0.284 & \textbf{0.355} \\
          & \multicolumn{1}{c|}{} & RMSE↓ & \underline{0.669} & 0.977 & 0.697 & 1.266 & 0.798 & 0.727 & \textbf{0.665} & 0.731 & 0.753 \\
    \midrule
    \multirow{6}[2]{*}{\rotatebox{90}{Chendu}} & \multicolumn{1}{c|}{\multirow{2}[1]{*}{LPC}} & ACC@1↑ & 0.563 & 0.552 & 0.394 & 0.531 & \textbf{0.616} & 0.423 & \underline{0.614} & 0.567 & 0.418 \\
          & \multicolumn{1}{c|}{} & F1↑   & 0.487 & 0.445 & 0.298 & 0.417 & \textbf{0.552} & 0.272 & \underline{0.548} & 0.499 & 0.274 \\
          & \multicolumn{1}{c|}{\multirow{2}[0]{*}{FI}} & MAE↓  & \textbf{147.8} & 164.2 & 156.1 & 171.9 & 174.3 & \underline{155.0} & 164.7 & 158.4 & 155.4 \\
          & \multicolumn{1}{c|}{} & RMSE↓ & \textbf{406.4} & 690.0 & 443.5 & 566.9 & 596.8 & 442.5 & 469.7 & \underline{414.9} & 443.1 \\
          & \multicolumn{1}{c|}{\multirow{2}[1]{*}{MI}} & MAE↓  & 5.9   & 24.7  & 4.2   & 27.4  & 307.3 & \underline{3.6} & 6.2   & 83.0  & \textbf{3.6} \\
          & \multicolumn{1}{c|}{} & RMSE↓ & \textbf{29} & 175   & \underline{30} & 768   & 2096  & 30    & 30    & 198   & 30 \\
    \midrule
    \multirow{6}[2]{*}{\rotatebox{90}{Xi'an}} & \multicolumn{1}{c|}{\multirow{2}[1]{*}{LPC}} & ACC@1↑ & 0.625 & 0.638 & 0.476 & 0.585 & \underline{0.664} & 0.504 & 0.603 & \textbf{0.674} & 0.512 \\
          & \multicolumn{1}{c|}{} & F1↑   & 0.476 & 0.531 & 0.278 & 0.427 & \textbf{0.601} & 0.293 & 0.461 & \underline{0.565} & 0.306 \\
          & \multicolumn{1}{c|}{\multirow{2}[0]{*}{FI}} & MAE↓  & 177.0 & 184.6 & \textbf{133.9} & 190.1 & 303.7 & \underline{133.9} & 241.8 & 148.6 & 134.3 \\
          & \multicolumn{1}{c|}{} & RMSE↓ & 964   & 941   & \textbf{327} & 1311  & 1730  & \underline{327} & 2169  & 697   & 327 \\
          & \multicolumn{1}{c|}{\multirow{2}[1]{*}{MI}} & MAE↓  & 3.4   & 494.7 & \underline{2.8} & 3.9   & 525.6 & 2.9   & 3.9   & 22.2  & \textbf{2.7} \\
          & \multicolumn{1}{c|}{} & RMSE↓ & 18    & 2067  & \underline{18} & 22    & 3456  & \textbf{18} & 22    & 106   & 18 \\
    \midrule
    \multirow{6}[2]{*}{\rotatebox{90}{Porto}} & \multicolumn{1}{c|}{\multirow{2}[1]{*}{LPC}} & ACC@1↑ & 0.357 & 0.339 & 0.257 & \textbf{0.374} & 0.357 & 0.292 & 0.357 & \underline{0.363} & 0.298 \\
          & \multicolumn{1}{c|}{} & F1↑   & 0.339 & 0.332 & 0.234 & \textbf{0.365} & 0.352 & 0.279 & 0.342 & \underline{0.353} & 0.295 \\
          & \multicolumn{1}{c|}{\multirow{2}[0]{*}{FI}} & MAE↓  & 223.4 & \textbf{194.1} & 516.8 & 245.2 & 248.4 & 515.9 & \underline{215.2} & 217.5 & 517.3 \\
          & \multicolumn{1}{c|}{} & RMSE↓ & 283.7 & \textbf{257.5} & 589.8 & 327.5 & 377.9 & 588.5 & \underline{273.9} & 305.0 & 590.4 \\
          & \multicolumn{1}{c|}{\multirow{2}[1]{*}{MI}} & MAE↓  & 22.64 & \textbf{19.91} & 44.82 & 21.98 & 20.97 & 44.78 & 22.33 & \underline{20.82} & 44.79 \\
          & \multicolumn{1}{c|}{} & RMSE↓ & 38.44 & \underline{30.15} & 72.23 & 38.44 & 31.56 & 72.19 & 39.79 & \textbf{29.92} & 72.19 \\
    \midrule
    \multirow{6}[2]{*}{\rotatebox{90}{San Francisco}} & \multicolumn{1}{c|}{\multirow{2}[1]{*}{LPC}} & ACC@1↑ & \textbf{0.827} & \underline{0.826} & 0.819 & 0.816 & 0.818 & 0.820 & 0.822 & 0.823 & 0.825 \\
          & \multicolumn{1}{c|}{} & F1↑   & \textbf{0.504} & 0.479 & 0.450 & 0.454 & 0.450 & 0.452 & 0.479 & \underline{0.504} & 0.502 \\
          & \multicolumn{1}{c|}{\multirow{2}[0]{*}{FI}} & MAE↓  & 462.0 & \underline{394.3} & 466.0 & 424.4 & 450.0 & 526.4 & \textbf{382.2} & 425.3 & 471.5 \\
          & \multicolumn{1}{c|}{} & RMSE↓ & 902   & \underline{802} & 872   & 819   & 910   & 1233  & \textbf{764} & 817   & 880 \\
          & \multicolumn{1}{c|}{\multirow{2}[1]{*}{MI}} & MAE↓  & 7.015 & \textbf{6.679} & 12.050 & 6.913 & 6.989 & 7.141 & \underline{6.714} & 6.840 & 7.061 \\
          & \multicolumn{1}{c|}{} & RMSE↓ & 22.30 & \underline{22.00} & 28.07 & 22.15 & 22.17 & 22.59 & \textbf{21.86} & 22.05 & 22.53 \\
    \midrule
    \multirow{2}{*}{Overall} & \multicolumn{2}{c|}{Per Ave Rank} & \textbf{3.677} & 4.452 & 5.935 & 5.161 & 5.355 & 5.871 & 4.097 & \underline{3.968} & 5.548 \\
          & \multicolumn{2}{c|}{Per Rank} & \textbf{1} & 4     & 9     & 5     & 6     & 8     & 3     & \underline{2} & 7 \\
    \bottomrule
    \end{tabular}%
    }
  \label{tab:land_parcel_comb}
\end{table}

\begin{table*}
  \centering
  \caption{Performance comparison of pretraining task combinations for segment across various datasets.}
      \resizebox{0.85\linewidth}{!}{
      \setlength{\tabcolsep}{0.5mm}
     \setlength{\extrarowheight}{-1pt}
            \begin{tabular}{c|cc|ccc|ccc|ccc|ccc|ccc|ccc}
    \toprule
    \multicolumn{3}{c|}{Token-based} & \multicolumn{9}{c|}{TokRI}                                            & \multicolumn{9}{c}{TRCL} \\
\cmidrule{1-21}    \multicolumn{3}{c|}{Graph-based} & \multicolumn{3}{c|}{NFI} & \multicolumn{3}{c|}{GAu} & \multicolumn{3}{c|}{AGCL} & \multicolumn{3}{c|}{NFI} & \multicolumn{3}{c|}{GAu} & \multicolumn{3}{c}{AGCL} \\
\cmidrule{1-21}    \multicolumn{3}{c|}{Sequence-based} & TrajP & MTR   & ATrCL & TrajP & MTR   & ATrCL & TrajP & MTR   & ATrCL & TrajP & MTR   & ATrCL & TrajP & MTR   & ATrCL & TrajP & MTR   & ATrCL \\
    \midrule
    \multirow{6}[2]{*}{\rotatebox{90}{Beijing}} & \multicolumn{1}{c|}{\multirow{2}[1]{*}{ASI}} & MAE↓  & 2.809 & 2.787 & 2.831 & 2.819 & 2.816 & 2.816 & 2.823 & 2.816 & 2.817 & 2.803 & 2.791 & \textbf{2.089} & 2.809 & 2.811 & 2.810 & \underline{2.310} & 2.771 & 2.790 \\
          & \multicolumn{1}{c|}{} & RMSE↓ & 5.483 & 5.461 & 5.489 & 5.492 & 5.485 & 5.485 & 5.487 & 5.485 & 5.489 & 5.475 & 5.464 & \textbf{4.731} & 5.487 & 5.486 & 5.487 & \underline{4.984} & 5.460 & 5.474 \\
          & \multicolumn{1}{c|}{\multirow{2}[0]{*}{TTE}} & MAE↓  & 609.1 & 636.2 & 644.5 & 634.8 & 598.1 & 608.6 & 577.9 & \textbf{511.4} & 578.2 & 692.7 & 776.7 & 542.6 & 575.1 & 613.8 & 594.4 & \underline{514.0} & 616.8 & 595.9 \\
          & \multicolumn{1}{c|}{} & RMSE↓ & 2592  & 2660  & 2597  & 2646  & 2587  & 2615  & 2493  & 2390  & 2518  & 2668  & 2722  & \textbf{2025} & 2591  & 2553  & 2572  & \underline{2214} & 2657  & 2624 \\
          & \multicolumn{1}{c|}{\multirow{2}[1]{*}{STS}} & ACC@3↑ & 0.961 & 0.944 & 0.531 & 0.269 & 0.356 & 0.783 & 0.912 & 0.361 & 0.808 & 0.949 & 0.977 & 0.793 & 0.957 & \textbf{0.980} & 0.702 & 0.915 & \underline{0.978} & 0.821 \\
          & \multicolumn{1}{c|}{} & MR↓   & 7.06  & 5.50  & 28.33 & 30.27 & 18.98 & 10.54 & 12.42 & 19.93 & 9.42  & 9.71  & \textbf{5.18} & 11.28 & 9.27  & \underline{5.34} & 13.87 & 10.10 & 5.50  & 9.12 \\
    \midrule
    \multirow{6}[2]{*}{\rotatebox{90}{Chendu}} & \multicolumn{1}{c|}{\multirow{2}[1]{*}{ASI}} & MAE↓  & 6.304 & 6.215 & 6.152 & 6.049 & 6.041 & \underline{5.999} & 6.087 & \textbf{5.964} & 6.009 & 6.283 & 6.222 & 6.207 & 6.092 & 6.060 & 6.001 & 6.193 & 6.121 & 6.019 \\
          & \multicolumn{1}{c|}{} & RMSE↓ & 13.62 & 13.53 & 13.53 & 13.45 & 13.44 & 13.40 & 13.49 & \textbf{13.38} & 13.41 & 13.51 & 13.47 & 13.53 & 13.48 & 13.47 & \underline{13.40} & 13.49 & 13.41 & 13.43 \\
          & \multicolumn{1}{c|}{\multirow{2}[0]{*}{TTE}} & MAE↓  & 91.70 & \textbf{88.05} & 116.14 & 91.50 & 92.78 & 115.41 & \underline{88.73} & 91.98 & 93.62 & 89.73 & 88.91 & 148.14 & 89.75 & 92.09 & 90.93 & 90.13 & 90.27 & 99.14 \\
          & \multicolumn{1}{c|}{} & RMSE↓ & 143.1 & \textbf{141.1} & 168.7 & 144.6 & 147.0 & 168.4 & \underline{141.6} & 143.2 & 146.1 & 143.6 & 141.7 & 196.5 & 142.0 & 145.0 & 144.8 & 142.0 & 143.5 & 149.2 \\
          & \multicolumn{1}{c|}{\multirow{2}[1]{*}{STS}} & ACC@3↑ & 0.735 & 0.643 & 0.315 & 0.231 & 0.654 & 0.743 & \textbf{0.903} & 0.668 & 0.570 & 0.717 & 0.677 & 0.719 & 0.730 & 0.751 & 0.872 & 0.707 & 0.679 & \underline{0.873} \\
          & \multicolumn{1}{c|}{} & MR↓   & 15.40 & 14.68 & 35.58 & 67.72 & 11.75 & 11.26 & 10.62 & 14.94 & 14.77 & 14.07 & 14.53 & 12.21 & 15.33 & 13.07 & \textbf{9.98} & 13.87 & 13.59 & \underline{10.04} \\
    \midrule
    \multirow{6}[2]{*}{\rotatebox{90}{Xi'an}} & \multicolumn{1}{c|}{\multirow{2}[1]{*}{ASI}} & MAE↓  & 5.616 & 5.576 & 5.546 & 5.463 & 5.405 & 5.404 & 5.410 & 5.434 & \textbf{5.374} & 5.652 & 5.587 & 5.639 & 5.379 & 5.468 & \underline{5.378} & 5.411 & 5.438 & 5.410 \\
          & \multicolumn{1}{c|}{} & RMSE↓ & 11.04 & 11.02 & 11.05 & 10.95 & 10.94 & 10.94 & 10.92 & 10.93 & \textbf{10.87} & 11.01 & 10.99 & 11.05 & 10.91 & 11.01 & 10.90 & 10.95 & 10.90 & \underline{10.90} \\
          & \multicolumn{1}{c|}{\multirow{2}[0]{*}{TTE}} & MAE↓  & \textbf{117.1} & 119.6 & 202.7 & 119.5 & 189.8 & 128.1 & \underline{118.7} & 118.9 & 139.6 & 119.7 & 120.7 & 184.0 & 123.2 & 123.4 & 127.4 & 119.1 & 118.8 & 146.7 \\
          & \multicolumn{1}{c|}{} & RMSE↓ & 186.1 & 189.3 & 267.4 & 188.0 & 263.4 & 192.4 & \underline{186.1} & 188.7 & 208.6 & 187.4 & 188.5 & 250.5 & 192.2 & 191.2 & 197.3 & \textbf{185.7} & 188.3 & 215.4 \\
          & \multicolumn{1}{c|}{\multirow{2}[1]{*}{STS}} & ACC@3↑ & 0.776 & 0.714 & 0.349 & \underline{0.879} & 0.657 & 0.590 & \textbf{0.909} & 0.759 & 0.513 & 0.876 & 0.782 & 0.294 & 0.795 & 0.689 & 0.313 & 0.839 & 0.673 & 0.640 \\
          & \multicolumn{1}{c|}{} & MR↓   & 8.19  & 9.17  & 30.73 & \textbf{6.40} & 7.99  & 10.33 & 7.41  & 8.49  & 12.78 & 9.31  & 7.78  & 34.13 & \underline{6.53} & 12.47 & 31.37 & 6.87  & 14.08 & 12.10 \\
    \midrule
    \multirow{6}[2]{*}{\rotatebox{90}{Porto}} & \multicolumn{1}{c|}{\multirow{2}[1]{*}{ASI}} & MAE↓  & 4.307 & 4.307 & 4.287 & 4.276 & 4.288 & 4.310 & 4.266 & 4.263 & 4.269 & 4.332 & 4.320 & 4.302 & 4.294 & 4.285 & 4.276 & 4.284 & \underline{3.922} & \textbf{3.578} \\
          & \multicolumn{1}{c|}{} & RMSE↓ & 7.855 & 7.853 & 7.837 & 7.831 & 7.835 & 7.845 & 7.822 & 7.810 & 7.820 & 7.855 & 7.855 & 7.843 & 7.834 & 7.829 & 7.824 & 7.830 & \underline{7.493} & \textbf{7.152} \\
          & \multicolumn{1}{c|}{\multirow{2}[0]{*}{TTE}} & MAE↓  & 86.76 & 87.97 & 90.44 & 87.68 & 88.19 & 87.05 & 91.95 & 86.78 & 87.23 & 86.46 & 104.44 & 96.14 & 97.00 & 91.96 & 86.92 & 87.85 & \textbf{80.67} & \underline{80.84} \\
          & \multicolumn{1}{c|}{} & RMSE↓ & 133.1 & 133.9 & 135.1 & 134.6 & 133.4 & 133.2 & 136.2 & 132.7 & 133.6 & 133.4 & 156.7 & 144.5 & 140.1 & 136.3 & 132.5 & 132.3 & \underline{122.1} & \textbf{116.8} \\
          & \multicolumn{1}{c|}{\multirow{2}[1]{*}{STS}} & ACC@3↑ & 0.961 & 0.913 & 0.846 & 0.943 & \textbf{0.968} & 0.323 & 0.961 & 0.956 & 0.927 & 0.928 & 0.571 & 0.833 & 0.953 & \underline{0.965} & 0.962 & 0.959 & 0.951 & 0.778 \\
          & \multicolumn{1}{c|}{} & MR↓   & 6.67  & 8.00  & 9.55  & 7.36  & 6.97  & 22.11 & 6.66  & 6.83  & 7.10  & 7.06  & 18.53 & 9.26  & 7.97  & \textbf{6.57} & 6.74  & \underline{6.62} & 6.75  & 9.08 \\
    \midrule
    \multirow{6}[2]{*}{\rotatebox{90}{San Francisco}} & \multicolumn{1}{c|}{\multirow{2}[1]{*}{ASI}} & MAE↓  & 2.498 & 2.491 & \textbf{2.066} & 2.477 & 2.477 & 2.486 & 2.474 & 2.476 & \underline{2.473} & 2.494 & 2.494 & 2.494 & 2.477 & 2.476 & 2.475 & 2.478 & 2.478 & 2.478 \\
          & \multicolumn{1}{c|}{} & RMSE↓ & 5.368 & 5.364 & \textbf{4.893} & 5.360 & 5.359 & 5.365 & \underline{5.353} & 5.358 & 5.356 & 5.371 & 5.370 & 5.370 & 5.358 & 5.358 & 5.357 & 5.358 & 5.358 & 5.358 \\
          & \multicolumn{1}{c|}{\multirow{2}[0]{*}{TTE}} & MAE↓  &  406.7 & 371.7 & \textbf{289.4} & 461.1 & \underline{310.4} & 402.5 & 345.3 & 424.9 & 442.9 & 462.0 & 399.0 & 335.9 & 495.7 & 516.9 & 448.5 & 327.4 & 406.3 & 485.2\\
          & \multicolumn{1}{c|}{} & RMSE↓ &  2638  & 2618  & \textbf{1372} & 2592  & 2617  & 2607  & 2614  & 2656  & 2648  & \underline{2592} & 2619  & 2647  & 2668  & 2665  & 2662  & 2625  & 2647  & 2669 \\
          & \multicolumn{1}{c|}{\multirow{2}[1]{*}{STS}} & ACC@3↑ & 0.683 & 0.813 & 0.703 & 0.743 & 0.867 & 0.720 & \textbf{0.887} & 0.777 & 0.690 & 0.777 & 0.857 & 0.740 & 0.683 & 0.697 & 0.807 & 0.767 & 0.810 & \underline{0.880} \\
          & \multicolumn{1}{c|}{} & MR↓   & 9.000 & 7.500 & 9.367 & 8.200 & 7.400 & 8.600 & \textbf{5.900} & 8.367 & 8.067 & 8.900 & 7.967 & 10.167 & 9.200 & 7.833 & 7.933 & 8.233 & 7.833 & \underline{6.933} \\
    \midrule
    \multirow{2}{*}{Overall} & \multicolumn{2}{c|}{Per Ave Rank} & 10.19 & 9.90  & 13.03 & 10.52 & 9.45  & 10.61 & \textbf{6.13} & 8.06  & 9.71  & 10.39 & 10.58 & 12.19 & 9.81  & 9.23  & 8.32  & \underline{7.00} & 7.35  & 8.42 \\
          & \multicolumn{2}{c|}{Per Rank} & 12    & 11    & 18    & 14    & 8     & 16    & \textbf{1} & 4     & 9     & 13    & 15    & 17    & 10    & 7     & 5     & \underline{2} & 3     & 6 \\
    \bottomrule
    \end{tabular}%
    }
  \label{tab:road_segment_comb}
\end{table*}
\FloatBarrier

% \begin{figure}
%     \centering
%     \subfigure[Top 3 combinations for POI map entity.]{\includegraphics[width=0.33\columnwidth]{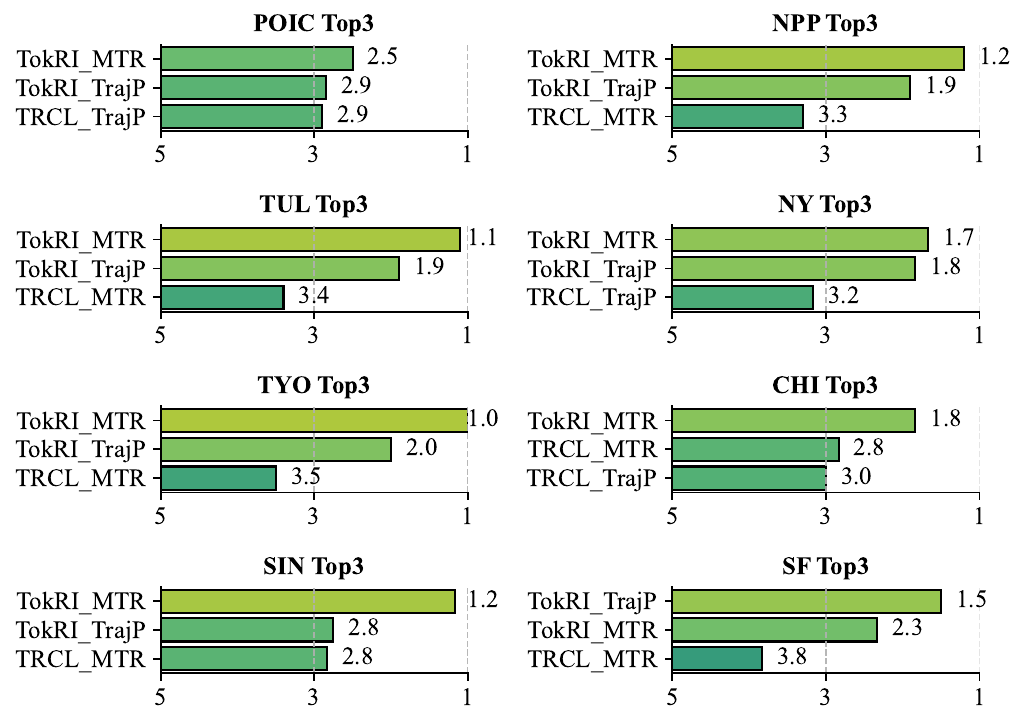}}
%     \subfigure[Top 3 combinations for segment map entity.]{\includegraphics[width=0.33\columnwidth]{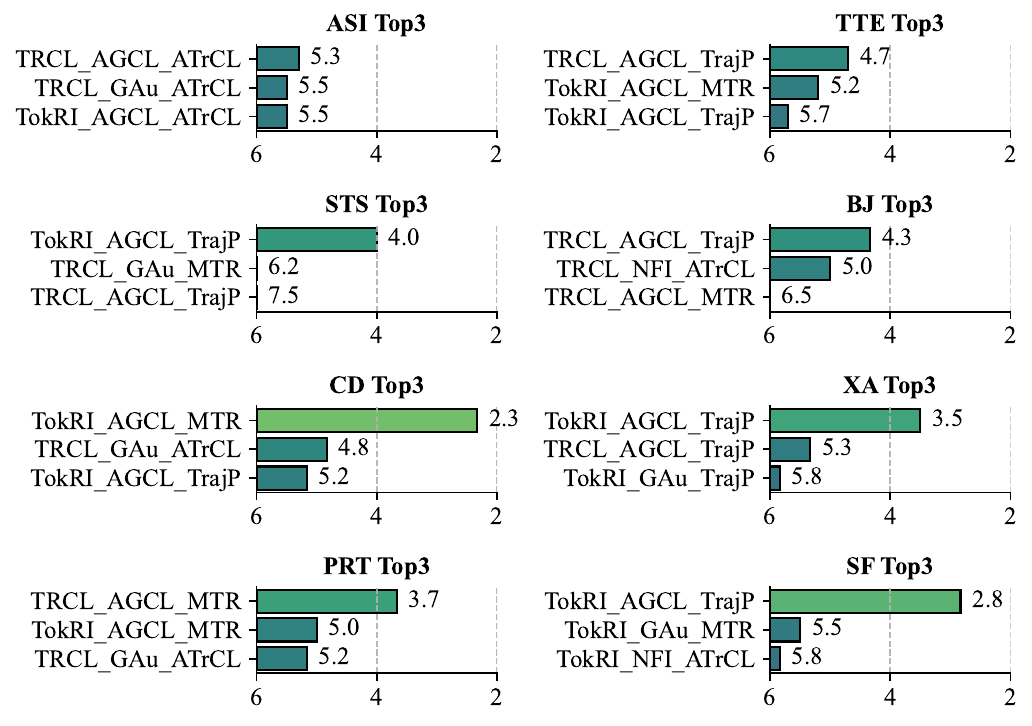}}
%     \subfigure[Top 3 combinations for parcel map entity.]{\includegraphics[width=0.33\columnwidth]{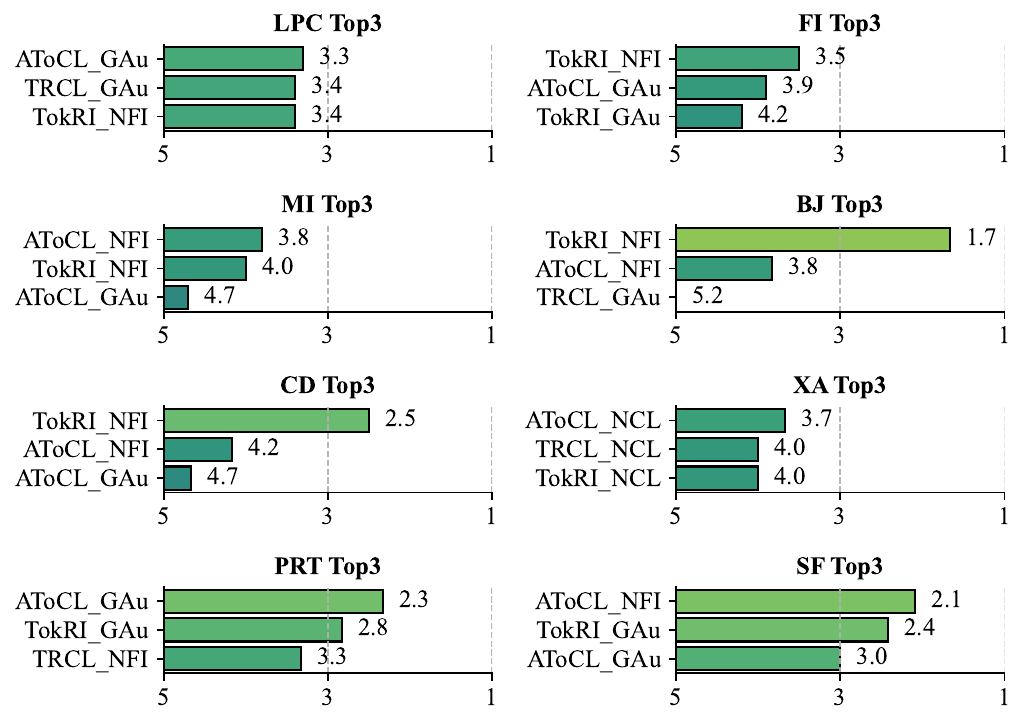}}
%     \vspace{-4mm}
%     \caption{Top 3 pretraining task combinations' preformance.}
%     \vspace{-4mm}
%     \label{fig:comb}
% \end{figure}

% By integrating these insights, we provide a general guide for selecting pretraining tasks across different entity types:

% 1) {\em Token-based}: Encoding semantic features is a key capability of token-based encoders. TokRI is well-suited for structured categorical attributes, while AToCL’s augmentation-based contrastive learning better handles high-dimensional and redundant semantic features, making it particularly effective for land parcels.

% 2) {\em Graph-based}: AGCL is well-suited for geographic relation networks, as it effectively captures key spatial dependencies. In contrast, GAu and NFI perform better in social relation networks due to their ability to model similarity-driven connectivity.

% 3) {\em Sequence-based}: MTR excels at capturing sequential dependencies, making it the best choice for sequence-based tasks, but it requires dense data to be effective. In contrast, TrajP is more reliable in sparse data scenarios.

\paratitle{Time Efficiency.}
In addition, we evaluate the training time efficiency of each pretraining task, with the results presented in \tab\ref{tab:compttime}. All time measurements are collected under the same computing environment as the performance experiments to ensure consistency. The convergence criterion is defined as the point where the loss approaches its minimum value and remains stable for at least 10 consecutive epochs. This criterion is applied uniformly across all pretraining tasks to ensure a fair comparison.
\begin{table*}
  \centering
  \small
  \caption{Time efficiency comparison for pretraining tasks. "Conver." is short for "Convergence" .}
  \resizebox{0.8\textwidth}{!}{
    \begin{tabular}{r|ccc|ccc|ccc|c}
    \toprule
    \multirow{2}[6]{*}{\makecell{Pretrining\\Task}} & \multicolumn{3}{c|}{POI} & \multicolumn{3}{c|}{Road Segment} & \multicolumn{3}{c|}{Land Parcel} & \multicolumn{1}{c}{\multirow{2}[6]{*}{\makecell{Relative\\Rank}}} \\
\cline{2-10}          & \multicolumn{1}{c}{\makecell{Step\\Time (ms)}} & \multicolumn{1}{c}{\makecell{Conver.\\Step}} & \multicolumn{1}{c|}{\makecell{Conver.\\Time (min)}} & \multicolumn{1}{c}{\makecell{Step\\Time (ms)}} & \multicolumn{1}{c}{\makecell{Conver.\\Step}} & \multicolumn{1}{c|}{\makecell{Conver.\\Time (min)}}& \multicolumn{1}{c}{\makecell{Step\\Time (ms)}} & \multicolumn{1}{c}{\makecell{Conver.\\Step}} & \multicolumn{1}{c|}{\makecell{Conver.\\Time (min)}}&  \\
    \midrule
    TokRI & 6.62 & 7367  & 1.0   & 197   & 31037 & 102   & 38    & 23840 & 15    & 2 \\
    TRCL  & 6.69 & 19100 & 2.2   & 307   & 28086 & 144   & 54    & 22387 & 20    & 3 \\
    AToCL & -     & -     & -     & -     & -     & -     & 4     & 23134 & 2     & 1 \\
    \midrule
    NFI   & -     & -     & -     & 223   & 29526 & 110   & 45    & 21192 & 16    & 2 \\
    NCL   & -     & -     & -     & -     & -     & -     & 45    & 20138 & 15    & 1 \\
    GAu   & -     & -     & -     & 264   & 32033 & 133   & 54    & 23943 & 22    & 3 \\
    AGCL  & -     & -     & -     & 289   & 28367 & 137   & -     & -     & -     & 4 \\
    \midrule
    TrajP & 18.81 & 15600 & 5.4   & 554   & 34152 & 315   & -     & -     & -     & 2 \\
    MTR   & 22.66 & 17050 & 7.2   & 1436  & 27483 & 658   & -     & -     & -     & 3 \\
    ATrCL & 25.14 & 6750  & 2.7   & 524   & 25800 & 225   & -     & -     & -     & 1 \\
    \bottomrule
    \end{tabular}%
    }
  \label{tab:compttime}%
\end{table*}%

From the results, we observe that AToCL, NCL, and ATrCL are the most computationally efficient pretraining tasks for token-based, graph-based, and sequence-based pre-training tasks, respectively. AToCL achieves the shortest convergence time among token-based pre-training tasks, making it the most efficient choice. For graph-based pretraining tasks, NCL converges the fastest, requiring fewer steps than NFI, which remains efficient but is slightly slower. In contrast, GAu and AGCL demand significantly more time, making them less favorable. Among sequence-based pretraining tasks, ATrCL is the most time-efficient, converging much faster than TrajP and MTR, with MTR being the slowest.
