# Supplementary material for: VecCity: A Taxonomy-guided Library for Map Entity Representation Learning
Source: arXiv:2411.00874 source file (2025-05-07)
Supplement: Supplementary file 2 [file appendix.tex]

\appendix

{\textbf{\Large Appendix}}

\section{Proofs}

\subsection{Derivation of $do$-operator using backdoor adjustment}\label{app:backdoor}

% using the following equation:
% \begin{equation}\small\label{apd:do}
%     P_{\Theta}(Y|do(X)) = \sum_{k=1}^{K}P_{\Theta}(Y|X, C=\mathcal{C}_k)P(C=\mathcal{C}_k).
% \end{equation}

The $do$-operator serves as a mathematical representation of an intervention, which is used to eliminate spurious correlations. In our approach, we utilize the backdoor adjustment to implement $P(Y|do(X))$ as in \equ~\eqref{eq:backdoor}. Before deriving it, we introduce two key rules of the $do$-operator proposed in \cite{2000Causality}. Consider variables $X$, $Y$, and $Z$ in a causal graph.
%based on our traffic causal graph in \fig~\ref{fig:scm}.

\begin{myappendixrule}\label{rule:a1}
    If variable $Z$ blocks all backdoor paths from $X$ to $Y$, then $do(X)$ is equivalent to $X$ when $Z$ is under control, 
    \begin{equation}
    P(Y|do(X),Z=z) = P(Y|X,Z=z). 
    \end{equation}
\end{myappendixrule}

A backdoor path represents a specific path between variable $X$ and variable $Y$, starting with an arrow pointing towards $X$, \eg $X \leftarrow Z \to Y$. The backdoor path serves as the underlying cause for the occurrence of spurious correlations between variables.

\begin{myappendixrule}\label{rule:a2}
    If there is no causal path between $X$ and $Y$, we can remove $do(X)$ from $P(Y|do(X))$,
    \begin{equation}
        P(Y|do(X)) = P(Y).
    \end{equation}
\end{myappendixrule}

In our traffic causal graph, ST context $C$ can affect $X$ and $Y$. Therefore, we can calculate $P(Y|do(X))$ across all possible values of $C$. By employing the rules of probability marginalization and the chain rule for joint probabilities, we have:
\begin{equation}
    P_\Theta(Y|do(X))=\sum_{k=1}^{K}P_\Theta(Y|do(X),C=\mathcal{C}_k)P(C=\mathcal{C}_k | do(X)).
\end{equation}
The right-hand side of this equation represents what we aim to estimate using only observational data. However, it contains two instances of $do(X)$ which hinder our estimation. 
Due to the fact that $C$ can block the only backdoor path $X \leftarrow C \rightarrow Y$, we can apply Rule A.\ref{rule:a1} to the first term of the right-hand side and have:
\begin{equation}
    P_\Theta(Y|do(X))=\sum_{k=1}^{K}P_\Theta(Y|X,C=\mathcal{C}_k)P(C=\mathcal{C}_k | do(X)).
\end{equation}

Then, the intervention $do(X)$ has cut the causal path between $X$ and $C$, allowing us to apply Rule A.\ref{rule:a2} and eliminate the $do(X)$ in the second term of the right-hand side. In this way, we arrive at the final equation:
\begin{equation}
    P_\Theta(Y|do(X))=\sum_{k=1}^{K}P_\Theta(Y|X,C=\mathcal{C}_k)P(C=\mathcal{C}_k).
\end{equation}

\subsection{Derivation of Rule \ref{rule:2}}\label{app:contional_dca}

% ${P(C=\mathcal{C}_{I_k})}/{P(C_{I})}=P(C_I = \mathcal{C}_{I_k})$
We derive Rule \ref{rule:2} through conditional probability, which is a measure of the probability of an event occurring, given that another event (by assumption, presumption, assertion or evidence) has already occurred~\footnote{\url{https://en.wikipedia.org/wiki/Sample_space}}. Next, we prove Rule \ref{rule:2} rigorously. 

Considering event $A = \{C=\mathcal{C}_{I_k}\}, I_k \in [I_1, I_K]$, and event $B=\{C=\mathcal{C}_{I_1}, C=\mathcal{C}_{I_2}, \dots, C=\mathcal{C}_{I_K}\} = \{C = \mathcal{C}_{I}\}$, we have $A \cap B = \{C=\mathcal{C}_{I_k}\} = A$. Therefore, the left term of the mentioned equation can be expressed as:

\begin{equation}
\begin{split}
\frac{P(C=\mathcal{C}_{I_k})}{P(C_{I})} =& \frac{P(A \cap B)}{P(B)}\\
=& P(A|B)\\
=& P(C=\mathcal{C}_{I_k}| C=\mathcal{C}_{I})\\
=& P(C=\mathcal{C}_{I_k}| C_I)\\
=& P(C_I = \mathcal{C}_{I_k})
\end{split}
\end{equation}

\subsection{Proof of Theorem \ref{thm:1}}\label{app:prf_thm1}
\begin{proof}
    Since each traffic context can be treated as invariant or variant according to its major membership, we can divide the context set of \equ~\eqref{eq:backdoor} into two groups and calculate them separately:
    \begin{equation}\small
        P_{\Theta}(Y|do(X)) = \sum_{I_k=I_1}^{I_K}P_{\Theta}(Y|X, C=\mathcal{C}_{I_k})P(C=\mathcal{C}_{I_k}) + \sum_{V_k=V_1}^{V_K}P_{\Theta}(Y|X, C=\mathcal{C}_{V_k})P(C=\mathcal{C}_{V_k})
    \end{equation}
    For each group, we introduce $P(C_{I})$ and $P(C_{V})$ respectively:
    \begin{equation}\small
    \begin{split}
        &P_{\Theta}(Y|do(X))\\
        =& \sum_{I_k=I_1}^{I_K}P_{\Theta}(Y|X, C=\mathcal{C}_{I_k})\frac{P(C=\mathcal{C}_{I_k})}{P(C_{I})}P(C_{I}) + \sum_{V_k=V_1}^{V_K}P_{\Theta}(Y|X, C=\mathcal{C}_{V_k})\frac{P(C=\mathcal{C}_{V_k})}{P(C_{V})}P(C_{V})\\
        =& P(C_{I}) \sum_{I_k=I_1}^{I_K}P_{\Theta}(Y|X, C=\mathcal{C}_{I_k})\frac{P(C=\mathcal{C}_{I_k})}{P(C_{I})} + P(C_{V}) \sum_{V_k=V_1}^{V_K}P_{\Theta}(Y|X, C=\mathcal{C}_{V_k})\frac{P(C=\mathcal{C}_{V_k})}{P(C_{V})}\\
        =& P(C_{I}) \sum_{I_k=I_1}^{I_K}P_{\Theta}(Y|X, C=\mathcal{C}_{I_k})P(C_I=\mathcal{C}_{I_k}) + P(C_{V}) \sum_{V_k=V_1}^{V_K}P_{\Theta}(Y|X, C=\mathcal{C}_{V_k})P(C_V=\mathcal{C}_{V_k})
    \end{split}
    \end{equation}
    The second step moves $P(C_{I})$ and $P(C_{V})$ to the outside of the summation symbol because they are constant \wrt indexing variables $I_k$ and $V_k$. The last step applies Rule \ref{rule:2}. Then, we apply the law of total probability to the above equation and obtain:
    \begin{equation}
        P_{\Theta}(Y|do(X)) = P(C_{I}) P_{\Theta}(Y|X, C=\mathcal{C}_{I})+ P(C_{V})P_{\Theta}(Y|X, C=\mathcal{C}_{V}).
    \end{equation}
    This means that we can treat all invariant/variant contexts as a whole to calculate their effect. We then can come to our proposed DCA in \equ~\eqref{eq:dca} by applying Rule \ref{rule:1}.
\end{proof}

% \section{Derivation of Upper Bound}\label{app:up_bound}

% In Section \ref{ssec:disent}, we try to estimate the mutual information between $\mathcal{Z}_I$ and $\mathcal{Z}_V$ via \eqref{eq:loss_m}. Here we provide an analysis 

\section{MSE Loss in Traffic Load Prediction}\label{app:mse}

Although traffic flow takes continuous values, it is not guaranteed that any possible value exists in the dataset and all values are uniformly distributed. It leads to the following challenges in the \emph{traffic load prediction} task: 

\begin{itemize}
    \item Firstly, when we discretize the traffic flow into 6 traffic load states, there may be some missing states. For example, given the historical maximum flow as 120, we can derive the 6 load states: $[0-20], [21-40], [41-60], [61-80], [81-100]$, and $[100, 120]$. However, there may be no data sampled from the state $[61-80]$. This leads to the classification task being difficult to converge, and the model cannot generate good predictions when there is a test sample located in the state $[61-80]$.
    \item Secondly, the non-uniformly distributed traffic flow data leads to a class imbalance issue, which makes the classification task suffer from poor generalization performance.
\end{itemize}

To solve these challenges, we propose to use the MSE loss function to penalize the difference between the forecasted and real traffic loads. The MSE loss also produces better empirical results.

\section{Dataset Statistics}\label{app:data}

There are four datasets in our experiments, including NYCBike1, NYCBike2, NYCTaxi, and BJTaxi. They are published in Ref.~\cite{ji2023spatio}. The statistics of these datasets are shown in \tab\ref{tab:SoD}. Since we aim to address the network-based ST traffic forecasting problem, we treat regions as network nodes. 

% Table generated by Excel2LaTeX from sheet 'dataset'
\begin{table}[htbp]
  \centering
  \caption{Statistics of Datasets}
    \begin{tabular}{rcccc}
    \toprule
    Dataset & NYCBike1 & NYCBike2 & NYCTaxi & BJTaxi \\
    \midrule
    Time interval & 1 hour & 30 min & 30 min & 30 min \\
    \# regions & 16$\times$8  & 10$\times$20 & 10$\times$20 & 32$\times$32 \\
    \# taxis/bikes & 6.8k+ & 2.6m+ & 22m+  & 34k+ \\
    \# seq length & 4392  & 2880  & 2880  & 5596 \\
    \bottomrule
    \end{tabular}%
  \label{tab:SoD}%
\end{table}%

\section{Implementation Details}\label{app:baseline}

Before we delve into the implementation details of baselines, we explain our evaluation metrics. We use two metrics to measure the performance of predictive models. We use $\bm{Y}^{(i)} \in \mathbb{R}^{N \times 2}$ to denote the ground truth of network-based traffic flow at time step $i$, and $\hat{\bm{Y}}^{(i)}$ to denote the predicted values. Consider there is a total of $M$ samples. We use $\Vert \cdot \Vert_1$ to denote the L1 norm. The metrics are defined as follows.

Mean Absolute Error (MAE):
\begin{equation}
    MAE=\frac{1}{M}\sum_{i=1}^{M} \left\Vert\bm{Y}^{(i)} - \hat{\bm{Y}}^{(i)}\right\Vert_{1}.
\end{equation}
% \begin{equation}
%     MAE=\frac{1}{2N}\sum_{i=1}^{N}\sum_{j=0}^1{|\bm{Y}_{i,j} - \hat{\bm{Y}}_{i,j}|}.
% \end{equation}

Mean Absolute Percentage Error (MAPE):
\begin{equation}
    MAPE=\frac{1}{M} \sum_{i=1}^{M} \left\Vert\frac{\bm{Y}^{(i)} - \hat{\bm{Y}}^{(i)}}{\bm{Y}^{(i)}}\right\Vert_{1}.
\end{equation}

% \begin{equation}
%     MAPE=\frac{1}{2N} \sum_{i=1}^{N} \sum_{j=0}^1\left(\frac{|\bm{Y}_{i,j} - \hat{\bm{Y}}_{i,j}|}{\bm{Y}_{i,j}}\right).
% \end{equation}
% where $\hat{\bm{Y}}_{i,j}$ represents the prediction result of $i$-th node and $j$-th type of flow. Likewise, $\bm{Y}_{i,j}$ denotes its ground truth.

The details of the baselines are as follows:
\begin{itemize}
    \item COST: it is a contrastive learning method for disentangled seasonal-trend representation learning in time series forecasting. We adapt this method to the spatial-temporal traffic forecasting problem by treating traffic data as multivariate time series. Following the code released by the original paper, we set the representation dimension to 320 and the learning rate to 0.001 for all datasets.
    \item STGCN: it consists of two spatial-temporal convolutional blocks, one temporal convolutional layer, and one output layer. We set the size of the temporal kernel to 3, the order of Chebyshev polynomials to 3, and the filter number to 128 for both CNN and GCN. Besides, the learning rate is set to 0.001 for all datasets.   
    \item AGCRN: it uses an adaptive adjacency metric to capture node-specific spatial dynamics, eliminating the need for pre-defined adjacency matrices. We implemented AGCRN using the released code. We set the RNN hidden unit number to 64 and the node embedding dimension to 10. 
    \item ASTGNN: it employs the transformer framework for traffic forecasting. It incorporates several self-attention blocks to model the dynamics of traffic data in both temporal and spatial dimensions. We utilize the released code for implementation. The initial learning rate is 0.001 and the dimension of hidden representations is 64. The head number of the attention layer is 8.
    \item ST-Norm: it introduces two types of normalization modules, namely temporal normalization and spatial normalization, to refine the high-frequency and local components of the original data, respectively. We implemented ST-Norm using the code released in the original paper. The hidden channel of the graph convolution is 16, and the learning rate is 0.0001.
    \item GTS: it enhances multivariate time series forecasting by leveraging graph structure learning. For implementation, we reuse the code and hyperparameters provided by the original paper. We set the hidden unit number to 64 and the kernel size to 10.
    \item STNSCM: it incorporates traffic flow with external conditions such as time factors, holidays, and weather information. In our fair comparison, we used time factors as input for the external conditions. We implemented STNSCM by reusing the code and hyperparameters released in the original paper. The depth of graph convolution is 2. The learning rate is 0.001 with a weight decay of 0.0001. The dimension of embedding dimension is 64.
\end{itemize}

\textbf{CaST:} We conduct a grid search for the representation dimension among $\{16, 32, 64, 128\}$. Ultimately, for the BJTaxi and NYCBike2 datasets, we set the representation dimension to 32, while for the NYCBike1 and NYCTaxi datasets, it is set to 64. Besides, the initial learning is set to 0.001 and we utilize a dynamic weight averaging strategy to balance the learning rate between multiple self-supervised tasks. We optimize our \model with the Adam optimizer. Please refer to the code at \git ~for more details.

\section{More Results of Temporal OOD Scenario}\label{app:t_ood_mape}

\tab\ref{tab:mape_temporal} presents the MAPE results for the baselines on datasets. We can observe similar phenomena as the results of MAE, \eg our \model surpasses other baselines in most cases, and AGCRN delivers the second-best performance.

% Table generated by Excel2LaTeX from sheet 'Sheet4'
\begin{table}[htbp]
  \centering
  \caption{Results of \emph{temporal OOD} setting on four datasets \wrt MAPE. We report an average of three runs. The title of each column indicates the test scenario. Column Avg. means the average result of all scenarios. The best results are highlighted with the bold font and the second with an underscore.}
  \setlength\tabcolsep{3pt}
  \setstretch{1.1}
  \resizebox{\linewidth}{!}{
    \begin{tabular}{c|cc|c|cc|c|cc|c|cc|c}
    \toprule
    \multirow{2}[2]{*}{Datasets} & \multicolumn{3}{c|}{NYCBike1} & \multicolumn{3}{c|}{NYCBike2} & \multicolumn{3}{c|}{NYCTaxi} & \multicolumn{3}{c}{BJTaxi} \\
    \cmidrule{2-13}
    \multicolumn{1}{c|}{} & Workday & Holiday & Avg.  & Workday & Holiday & Avg.  & Workday & Holiday & Avg.  & Workday & Holiday & Avg. \\
    \midrule
    COST  & 29.67  & 37.62  & 33.65  & 31.23  & 39.32  & 35.28  & 32.80  & 30.37  & 31.59  & 17.10  & 22.41  & 19.76  \\
    \midrule
    STGCN & 25.28  & 29.98  & 27.63  & 25.09  & 30.71  & 27.90  & 18.90  & 18.69  & 18.80  & 14.91  & 19.34  & 17.13  \\
    AGCRN & \underline{25.19}  & 29.71  & 27.45  & 24.62  & 30.15  & 27.39  & \underline{18.28}  & \underline{17.99}  & \underline{18.14}  & \underline{14.68}  & 18.92  & \underline{16.80}  \\
    ASTGNN & 25.34  & 28.82  & 27.08  & 28.16  & 35.24  & 31.70  & 19.45  & 24.27  & 21.86  & 15.31  & 19.77  & 17.54  \\
    ST-Norm & 25.46  & \underline{26.45}  & \underline{25.96}  & 26.25  & \underline{27.62}  & 26.94  & 31.47  & 30.55  & 31.01  & 16.75  & \textbf{18.27} & 17.51  \\
    \midrule
    GTS   & 25.54  & 30.27  & 27.91  & \underline{24.22}  & 29.02  & \underline{26.62}  & 18.35  & 18.60  & 18.48  & 17.15  & 21.49  & 19.32  \\
    STNSCM & 26.67  & 29.91  & 28.29  & 27.88  & 31.13  & 29.51  & 23.63  & 23.39  & 23.51  & 16.96  & 19.36  & 18.16  \\
    CaST  & \textbf{22.63} & \textbf{26.17} & \textbf{24.40} & \textbf{20.54} & \textbf{24.61} & \textbf{22.58} & \textbf{16.72} & \textbf{16.25} & \textbf{16.49} & \textbf{14.20}  & \underline{18.90}  & \textbf{16.55} \\
    \bottomrule
    \end{tabular}%
    }
  \label{tab:mape_temporal}%
\end{table}%

\section{More Results of Spatial OOD Scenario}\label{app:s_ood_result}

\subsection{Clustering Visualization}\label{app:cluster}

We provide the clustering results on the other three datasets in \fig~\ref{fig:cluster}.

\begin{figure}[!ht]
    \centering
    \subfigure[NYCBike1]{\includegraphics[width=0.25\columnwidth]{figures/cluster/NYCBike1.pdf}\label{fig:cluster_NYCBike1}
    }~~~~~~
    \subfigure[NYCBike2]{\includegraphics[width=0.25\columnwidth]{figures/cluster/NYCBike2.pdf}\label{fig:cluster_NYCBike2}}~~~~~~
    \subfigure[NYCTaxi]{\includegraphics[width=0.25\columnwidth]{figures/cluster/NYCTaxi.pdf}\label{fig:cluster_NYCTaxi}}
    \caption{Spatial clustering results of different datasets. The cluster ID is next to the color bar. A larger cluster ID means a higher level of popularity.}\label{fig:cluster}
\end{figure}

\subsection{Performance Comparison \wrt MAPE}\label{app:s_ood_mape}

We also test the MAPE performance of our method and baselines under the spatial ood scenario, and the results are shown in \tab~\ref{tab:mape_spatial}. We can observe that our \model achieves the best average performance for all datasets.

% Table generated by Excel2LaTeX from sheet 'MAPE Spatial'
\begin{table}[htbp]
  \centering
  \caption{\emph{Spatial OOD} results on four datasets \wrt MAPE (\%). The ratio besides the dataset means the distribution of different clusters in training data. c0 means the cluster with ID 0, and so on.}
  \setlength\tabcolsep{3pt}
  \setstretch{1.1}
  \resizebox{\linewidth}{!}{
    \begin{tabular}{c|cccc|c|ccc|c|cccc|c|ccccc|c}
    \toprule
    \multirow{2}[2]{*}{Dataset} & \multicolumn{5}{c|}{NYCBike1 (6:2:1:1)} & \multicolumn{4}{c|}{NYCBike2 (8:1:1)} & \multicolumn{5}{c|}{NYCTaxi (15:2:2:1)}  & \multicolumn{6}{c}{BJTaxi (11:8:6:3:2)} \\
    \cmidrule{2-21}
    \multicolumn{1}{c|}{} & c0    & c1    & c2    & c3    & Avg.  & c0    & c1    & c2    & Avg.  & c0    & c1    & c2    & c3    & Avg.  & c0    & c1    & c2    & c3    & c4    & Avg. \\
    \midrule
    COST  & 31.43  & 32.16  & 33.65  & 29.67  & 31.73  & 36.68  & 31.92  & 33.54  & 34.05  & 31.11  & 33.55  & 34.19  & 33.07  & 32.98  & 23.76  & 18.62  & 15.91  & 14.50  & 12.94  & 17.15  \\
    \midrule
    STGCN & 33.86  & 28.50  & 24.56  & 22.28  & 27.30  & 37.47  & 26.47  & \underline{20.17}  & 28.04  & 27.68  & 16.80  & 11.42  & 9.74  & 16.41  & 23.88  & 15.41  & 12.38  & 10.56  & 9.34  & 14.31  \\
    AGCRN & 33.46  & 28.88  & 25.41  & 22.61  & 27.59  & 36.73  & 26.04  & 19.75  & 27.51  & 26.14  & \underline{16.76}  & 11.34  & 9.65  & \underline{15.97}  & 28.87  & 15.37  & 12.77  & 11.46  & 9.29  & 15.55  \\
    ASTGNN & 34.18  & 28.55  & 25.19  & 22.93  & 27.71  & 37.62  & 27.86  & 22.06  & 29.18  & 33.39  & 17.44  & 11.48  & 9.63  & 17.98  & \underline{22.99}  & \textbf{14.56}  & \textbf{11.77}  & 10.90  & 9.53  & \underline{13.95}  \\
    ST-Norm & 33.29  & 27.42  & 24.31  & 21.26  & 26.57  & 33.33  & 28.86  & 21.42  & 27.87  & 45.77  & 30.53  & 18.23  & 16.37  & 27.72  & 25.63  & 16.87  & 13.38  & 10.79  & \underline{8.99}  & 15.13  \\
    \midrule
    GTS   & 34.82  & 28.69  & 25.08  & 21.99  & 27.64  & 33.40  & \underline{25.87}  & 20.51  & \underline{26.59}  & 27.11  & 16.82  & \textbf{11.01 } & \underline{9.36}  & 16.08  & 27.13  & 17.24  & 14.23  & 12.35  & 10.71  & 16.33  \\
    STNSCM & \underline{26.84}  & \underline{27.00}  & \textbf{22.13 } & \textbf{20.24 } & \underline{24.05}  & \underline{29.34}  & 27.52  & 28.18  & 28.35  & \underline{24.11}  & 22.65  & 12.43  & 11.11  & 17.58  & 23.87  & 18.43  & 14.22  & 12.22  & 9.64  & 15.67  \\
    CaST  & \textbf{23.90} & \textbf{26.80} & \underline{23.23}  & \underline{20.69}  & \textbf{23.66} & \textbf{24.04} & \textbf{23.57} & \textbf{18.70} & \textbf{22.10} & \textbf{22.46} & \textbf{16.36} & \underline{11.14}  & \textbf{9.16} & \textbf{14.78} & \textbf{22.87} & \underline{15.30} & \underline{12.10} & \textbf{10.18} & \textbf{8.78} & \textbf{13.85} \\
    \bottomrule
    \end{tabular}%
    }
  \label{tab:mape_spatial}%
\end{table}%

\subsection{Overall Performance Comparison and Nemenyi Test}\label{app:s_ood_test}
% TODO:
% 1. add tables of the win times and average rank for MAE and MAPE, respectively
% 2. carry out Nemenyi test for the above table with 5\% level

To further emphasize the substantial improvement of CaST over the baseline models, we statistic the average ranking of each model and count its win times, \ie the number of times a model performs best. As the results in \tab\ref{tab:win_rank_nemenyi}, \model achieves the best performance among all the competitors in terms of win times and average ranking.

% Table generated by Excel2LaTeX from sheet 'Nemenyi'
% \begin{table}[htbp]\small
%   \centering
%   \caption{Nemenyi test for Sptaial OOD Scenario. "Wins" indicates the number of times model achieve the best performance, "Avg. Rank" represents the average ranking obtained by the baseline model. Furthermore, the "test (\%)" indicates the significance level of the Nemenyi test with \model}
%     \begin{tabular}{c|cc|c|cc|c}
%     \toprule
%     \multirow{2}[2]{*}{Metric} & \multicolumn{3}{c|}{MAE} & \multicolumn{3}{c}{MAPE} \\
%           & Wins  & Avg. Rank & test(\%) & Wins  & \multicolumn{1}{c}{Avg. Rank} & \multicolumn{1}{c}{test(\%)} \\
%     \midrule
%     COST  & 0     & 7.00  & 0.10  & 0     & 7.01  & 0.10  \\
%     \midrule
%     STGCN & 0     & 3.81  & 4.99  & 0     & 4.25  & 1.25  \\
%     AGCRN & 0     & 4.37  & 0.50  & 0     & 4.44  & 0.57  \\
%     ASTGNN & 0     & 4.62  & 0.16  & 2     & 4.88  & 0.10  \\
%     ST-Norm & 1     & 5.31  & 0.10  & 0     & 4.88  & 0.10  \\
%     \midrule
%     GTS   & 0     & 4.25  & 1.10  & 1     & 4.88  & 0.10  \\
%     STNSCM & 2     & 5.43  & 0.10  & 2     & 4.38  & 0.74  \\
%     CaST  & \textbf{13} & \textbf{1.19} & 100   & \textbf{11} & \textbf{1.30} & 100  \\
%     \bottomrule
%     \end{tabular}%
%   \label{tab:win_rank_nemenyi}%
% \end{table}%

% Table generated by Excel2LaTeX from sheet 'Nemenyi'
\begin{table}[ht]\small
  \centering
  \caption{Summary of performance comparison in the spatial OOD scenario. ``Win times'' indicates the number of times a model achieves the best performance, ``Average ranking'' represents the average ranking of each model.}
  \resizebox{0.9\linewidth}{!}{
    \begin{tabular}{c|c|c|cccc|ccc}
    \toprule
    \multicolumn{2}{c|}{Method} & COST  & STGCN & AGCRN & ASTGNN & ST-Norm & GTS   & STNSCM & CaST \\
    \midrule
    \multirow{2}{*}{MAE} & Win times  & 0     & 0     & 0     & 0     & 1     & 0     & 2     & \textbf{13} \\
          & Average ranking & 7.00  & 3.81  & 4.37  & 4.62  & 5.31  & 4.25  & 5.43  & \textbf{1.19} \\
    \midrule
    \multirow{2}{*}{MAPE} & Win times  & 0     & 0     & 0     & 2     & 0     & 1     & 2     & \textbf{11} \\
          & Average ranking & 7.01  & 4.25  & 4.44  & 4.88  & 4.88  & 4.88  & 4.38  & \textbf{1.30} \\
    \bottomrule
    
    \end{tabular}%
    }
  \label{tab:win_rank_nemenyi}%
\end{table}%

\begin{figure}[ht]
    \centering
    \subfigure[CD diagram of MAE metric]{
        \includegraphics[width=0.45\linewidth]{figures/nemenyi1.pdf}
    }
    \quad
    \subfigure[CD diagram of MAPE metric]{
        \includegraphics[width=0.45\linewidth]{figures/nemenyi2.pdf}
    }
    \caption{Critical difference (CD) diagram of the spatial OOD experiments \wrt metrics MAE and MAPE. Blue lines correspond to spatio-temproal models using causality. Red lines correspond to graph-based spatial-temporal methods without causality. Yellow lines correspond to time series approaches.}
    \label{fig:nemenyi}
\end{figure}

% \tab\ref{tab:win_rank_nemenyi} provides the results of the Nemenyi test, which assesses the statistical significance of the performance differences. Based on these results, CaST demonstrates a significant improvement at a 5\% level of significance.

As shown in \fig~\ref{fig:nemenyi}, we also perform a Nemenyi test for the spatial OOD experiment results. On the Nemenyi critical difference diagrams, two methods have a statistically significant difference if the difference between their average
ranks is larger than the critical difference (the line segment with ``CD'' on the top left corner of the diagrams). Models that are connected by a bold line do not have a statistically significant difference. The performance of \model is significantly better than all baselines with a 5\% significance level.

\section{More Results of Model Analysis}

\subsection{Adaptation to Distribution Shifts}\label{app:prior}

\fig~\ref{fig:prior} shows the learned priors $\alpha_1$ and $\alpha_2$ on BJTaxi, which are corresponding to the invariant and variant ST contexts. We can observe quite different priors for workdays and holidays whose data distributions shifted a lot. 

% The data distribution of workdays and holidays are given in 

\begin{figure}[htbp]
    \centering
    \includegraphics[width=0.7\columnwidth]{figures/prior.pdf}
    \caption{Visualization of the learned priors. The horizontal axis represents the time of day. A brighter pixel means a larger value. }
    \label{fig:prior}
\end{figure}

\subsection{Ablation Study}\label{app:ablation}
To analyze the effectiveness of sub-modules in our CaST, we carry out ablation experiments on all four datasets with the following five variants:

\bul \textbf{CaST-CD:}  This variant disables the contextual disentangelment loss ($\mathcal{L}_D$).

\bul \textbf{CaST-Temporal:} This variant disables the temporal index identification self-supervised task ($\mathcal{L}_{ti}$).

\bul \textbf{CaST-Spatial:}  This variant disables the spatial location classification self-supervised task ($\mathcal{L}_{si}$).

\bul \textbf{CaST-Traffic:}  This variant disables the traffic load prediction self-supervised task ($\mathcal{L}_{tl}$).

\bul \textbf{CaST-GRL:}  This variant disables the gradient reversal layer in all self-supervised tasks.

\tab~\ref{tab:abl} presents the experimental results of our \model and its five variants, with each result representing the average performance of all temporal OOD scenarios. We can observe that: $i)$ The variants CaST-Temporal, CaST-Spatial, and CaST-Traffic perform worse than the original CaST model, suggesting that every self-supervised task plays an important role in improving performance. This observation also justifies the necessity of jointly modeling ST contexts from time, space, and traffic semantic perspectives. $ii)$ The variants CaST-CD and CaST-GRL deliver worse performance than the original model, indicating that decoupling $\mathcal{Z}_I$ and $\mathcal{Z}_V$ leads to a better OOD generalization. The reason is that maintaining a strong disentanglement between the two latent representations can satisfy the independence requirement of DCA, thus eliminating spurious correlations that impair OOD generalization. In summary, each designed sub-module has a positive effect on the performance improvement of our \model.

% Table generated by Excel2LaTeX from sheet 'Ablation'
\begin{table}[htbp]\small
  \centering
  \caption{Ablation study of our proposed \model.}
    \begin{tabular}{c|cc|cc|cc|cc}
    \toprule
    \multirow{2}[2]{*}{Dataset} & \multicolumn{2}{c|}{NYCBike1} & \multicolumn{2}{c|}{NYCBike2} & \multicolumn{2}{c|}{NYCTaxi} & \multicolumn{2}{c}{BJTaxi} \\
    \cmidrule{2-9}
          & MAE   & MAPE  & MAE   & MAPE  & MAE   & MAPE  & MAE   & MAPE \\
    \midrule
    CaST-CD & 5.05  & \underline{24.58}  & \underline{4.86}  & 23.16 & 10.74  & 17.18 & \underline{11.37} & \underline{16.68} \\
    CaST-Temporal & 5.08  & 25.38 & 4.89  & 23.47 & 11.04    & 17.36 & 11.43 & 16.89 \\
    CaST-Spatial & 5.07  & 24.87 & 4.89  & 23.18 & 10.67 & \underline{16.93} & 11.38 & 16.71 \\
    CaST-Traffic & 5.15  & 25.36 & 4.90   & \underline{22.67} & 10.61 & 17.42 & 11.48 & 16.73 \\
    CaST-GRL & \underline{5.04}  & 24.76 & 4.86  & 23.46 & \underline{10.60}  & 17.23 & 11.42 & 16.97 \\
    \midrule
    CaST  & \textbf{5.03} & \textbf{24.40} & \textbf{4.85} & \textbf{22.58} & \textbf{10.56} & \textbf{16.49} & \textbf{11.34} & \textbf{16.55} \\
    \bottomrule
    \end{tabular}%
  \label{tab:abl}%
\end{table}%

% \begin{itemize}
%     \item CaST achieves the best performance across all datasets, indicating the effectiveness of the model compared to the other variants.
%     \item The variants CaST-Temporal, CaST-Spatial, and CaST-Traffic perform worse than the original CaST model, suggesting that each self-supervised task plays an important role in improving performance. This observation also justifies the necessity of jointly modeling ST contexts from time, space, and traffic semantic perspectives.
%     \item The variants CaST-CD and CaST-GRL deliver worse performance than the original model, indicating that decoupling $\mathcal{Z}_I$ and $\mathcal{Z}_V$ leads to a better OOD generalization. The reason is that maintaining a strong disentanglement between the two latent representations can satisfy the independence requirement of DCA, thus eliminating spurious correlations that impair OOD generalization. 
%     % This results in a good generalization of \model to OOD traffic forecasting.
% \end{itemize}

% In summary, the experimental results demonstrate the effectiveness of the CaST model, the significance of the self-supervised tasks, and the benefits of preserving disentangling between the latent representations for improved out-of-distribution generalization.
